# Supplementary material for: Construction and testing of sMDT tubes at the University of Michigan for the ATLAS Muon Spectrometer upgrade
Source: arXiv:2209.03864 source file (2022-09-08)
Supplement: Supplementary file 1 [file Appendix.tex]

\section{Appendix: Gas Flushing Time Requirement} 
\label{sec:GasFlowTimeCalculation}
% A brief version of this calculation will be given in the Tube Testing 
% section and this appendix  will not be used in the paper. cjw
%
The amount of gas to be flushed to have a clean enough 
environment to apply HV is estimated to be 3 volumes. 
The gas flow rate bubbler units is standard cubic feet per 
hour (SCFH), allowing us to estimate the time needed to have 
a tube ready for the test.
\par
The volume of a single tube of outside diameter 15~mm is:
\begin{equation}
   V_{tube}= 1600\; mm \times \pi \times 7.1^{2} \; mm^{2}
   = 2.53 \times 10^{5} \; mm^{3}
   = 2.53 \times 10^{-4}\; m^{3}
\end{equation}

Each test station can be equipped with 48 tubes, leading to
\begin{equation}
    V_{total}= V_{tube}\times 48
    = 2.53 \times 48 \times 10^{-4}\; m^{3}
    = 1.22 \times 10^{-2}\; m^{3}
\end{equation}
The tube works at 31 psi higher than the atmospheric pressure, 
so by using the conversion 
$ \rm 1 \; psi = 6.805 \times 10^{-2} \; atm $,
the gas volume at running pressure is:
\begin{equation}
    V_{standard} = (1+31\times 6.805\times 10^{-2}) \times V_{total}
%    = 3.11 \times 1.31\times 10^{-2}\; m^{3}
    = 4.07\times 10^{-2}\; m^{3}
\end{equation}
The gas flow rate bubbler in MKS units is
\begin{equation}
    Rate = 1 \; SCFH = 0.3048^{3}\; m^{3}/h
    = 2.832 \times 10^{-2}\; m^{3}/h
\end{equation}
The total time for one volume at 1~SCFH:
\begin{equation}
    T_{0} = V_{standard}/Rate = 0.0407/0.02832 \; h = 
    1.44 \; h
\end{equation}
In the end, the total time to exchange 3 volumes of gas at 
31 psi above atmospheric pressure using a flow rate of 
1~SCHF is about 4.5 hours (or 1~h at 3~SCHF).
